# Supplementary material for: Characteristic time of stellar flares on Sun-like stars
Source: arXiv:2105.12375 ancillary file (2021-06-15)

# Plots of all the flare samples

April 25, 2021

This document includes all the light-curve plots of the 184 identified flare samples of Sun-like stars (SLS) observed in *Kepler* SC (short-cadence) mode. In each plot, the three vertical lines (from left to right) indicate the start, peak, and end times of the flare, respectively.

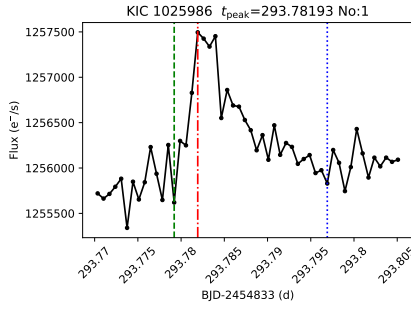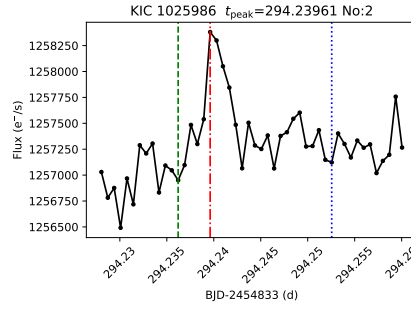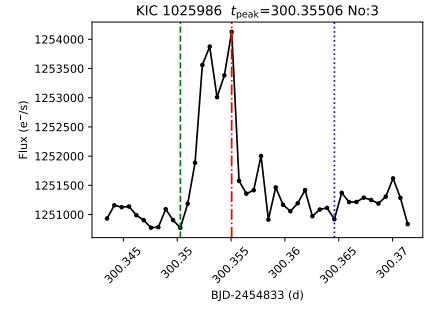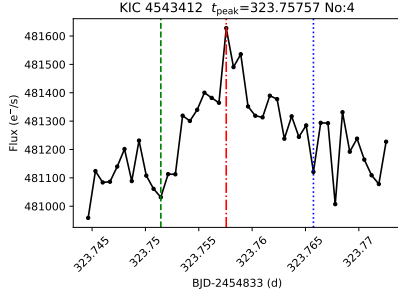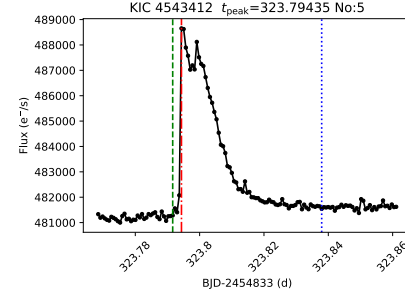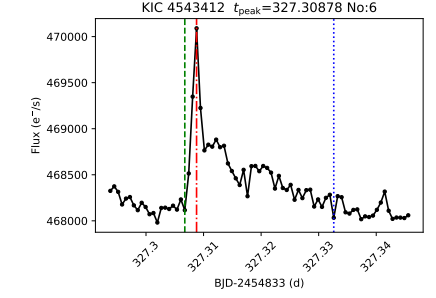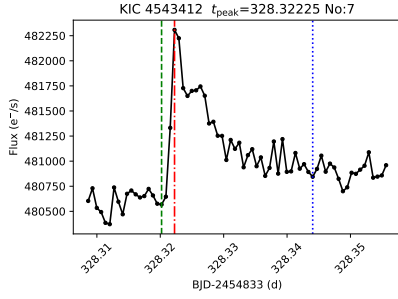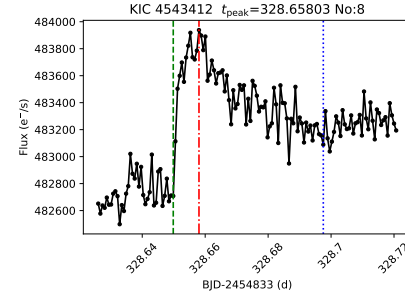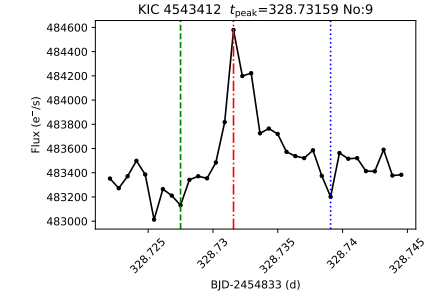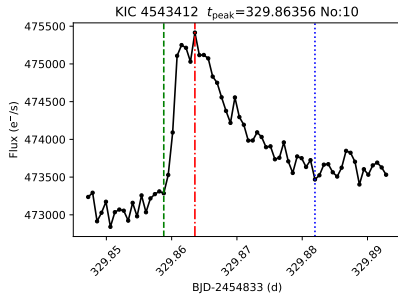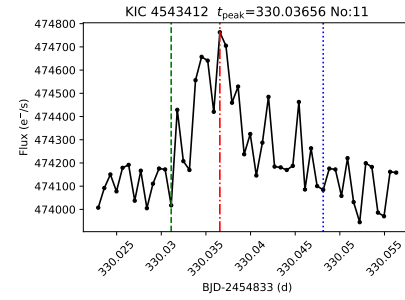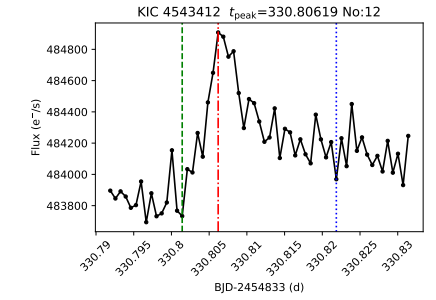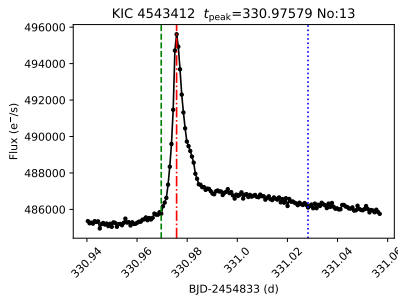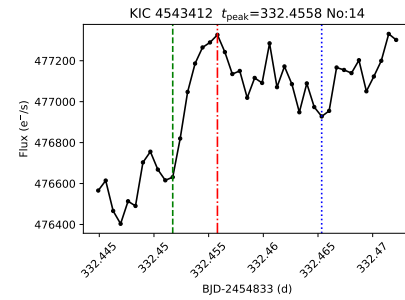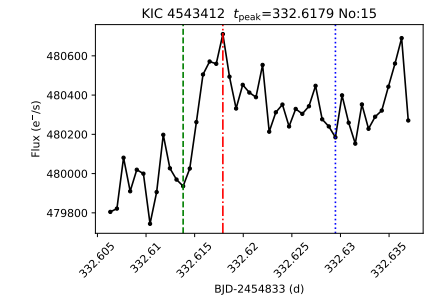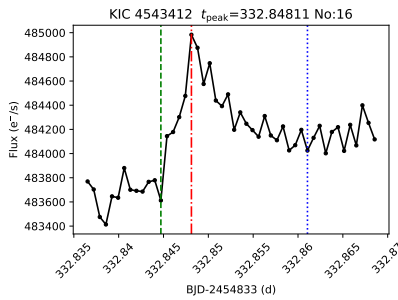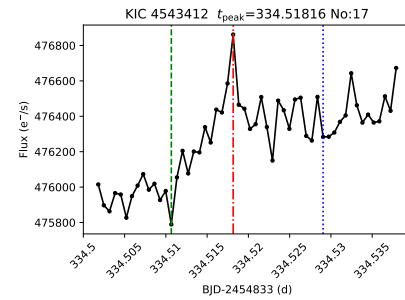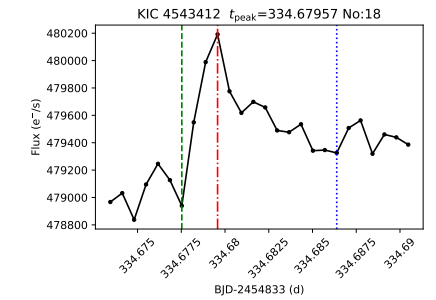

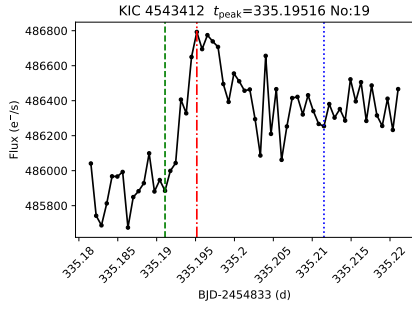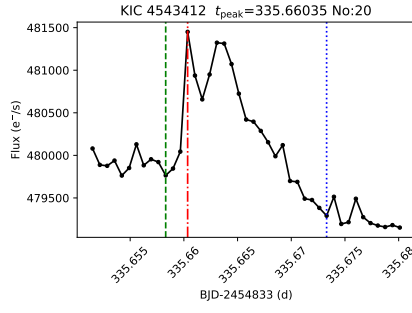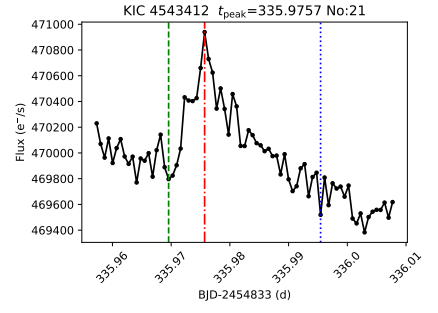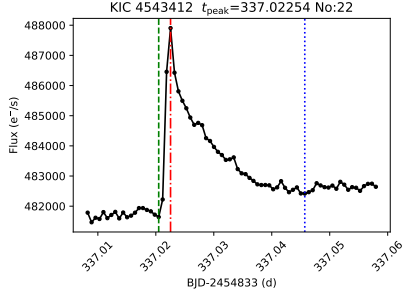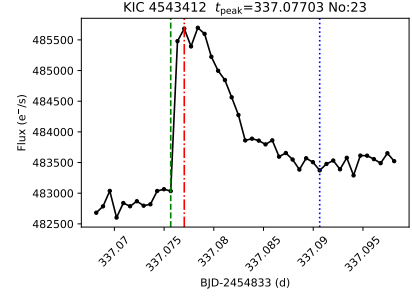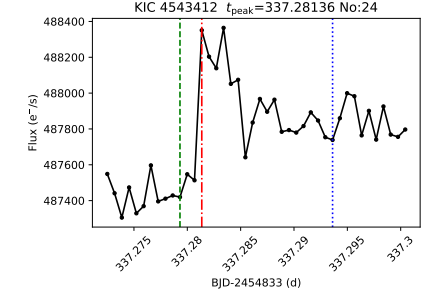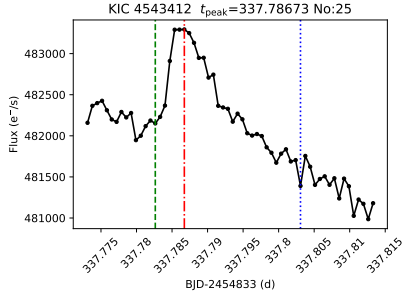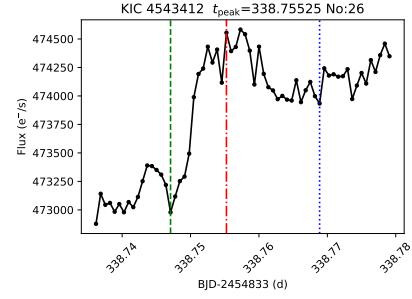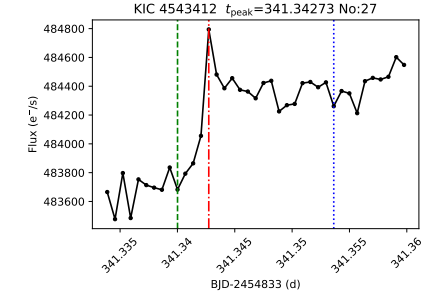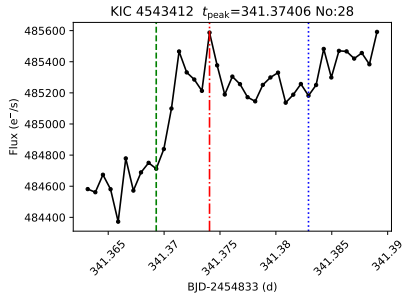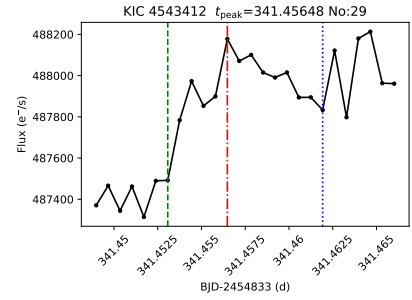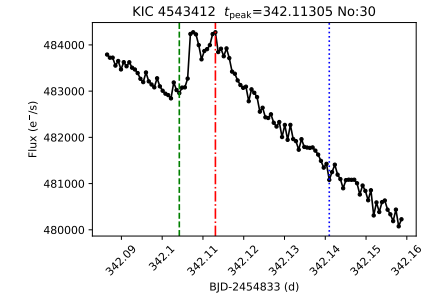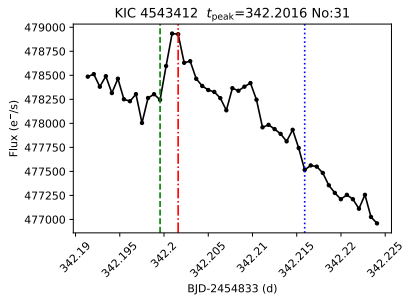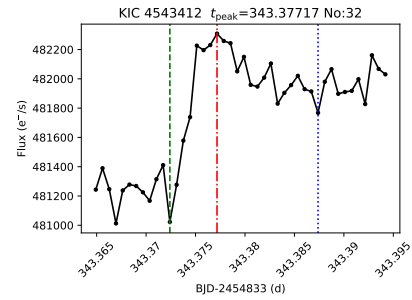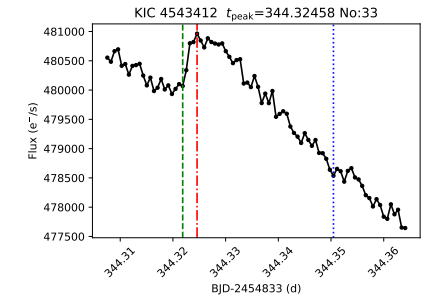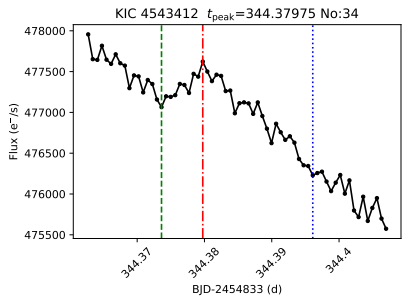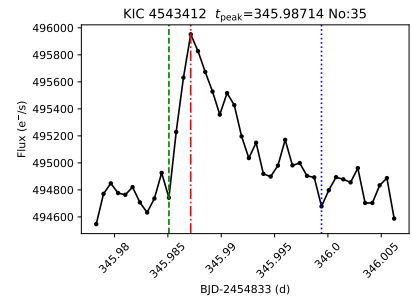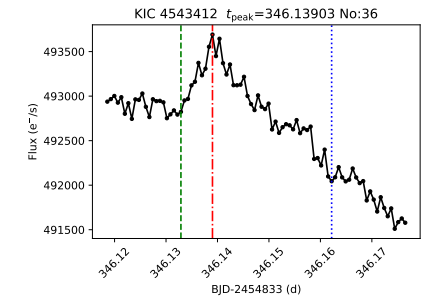

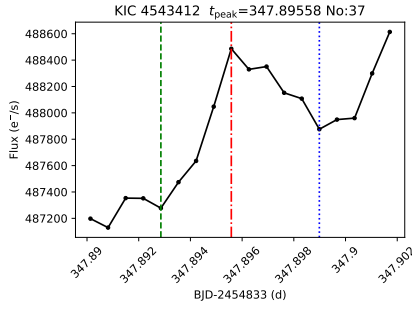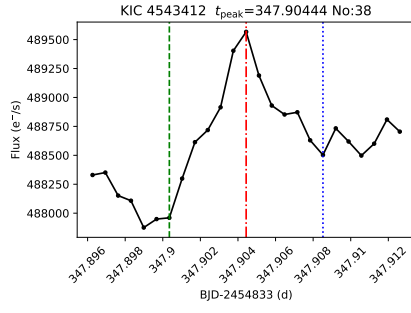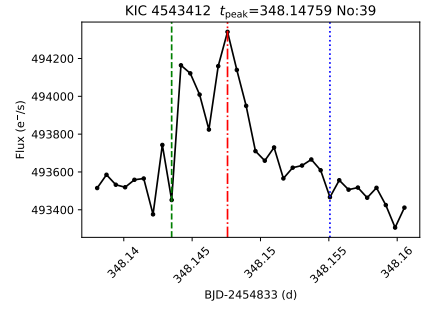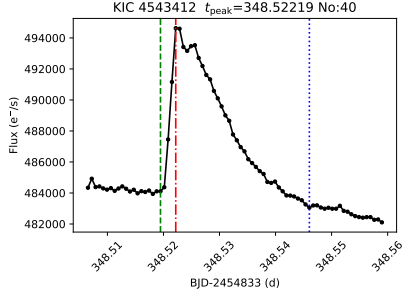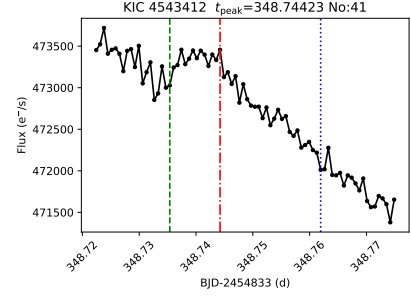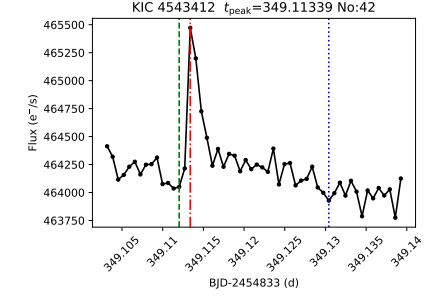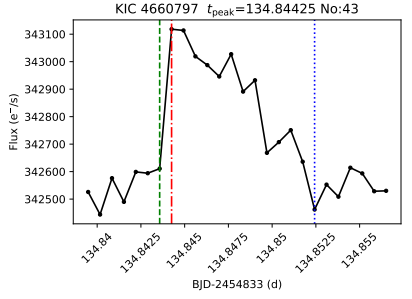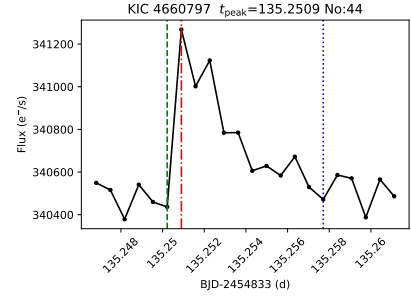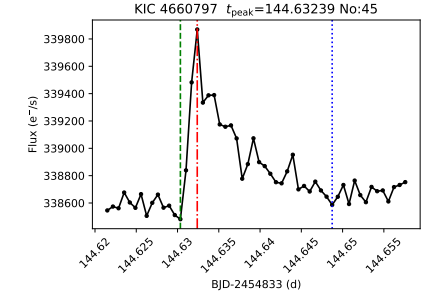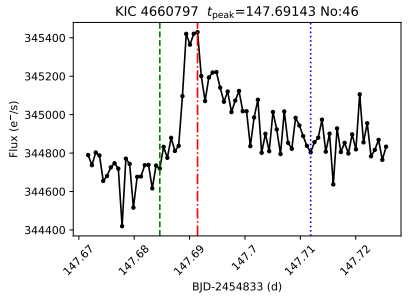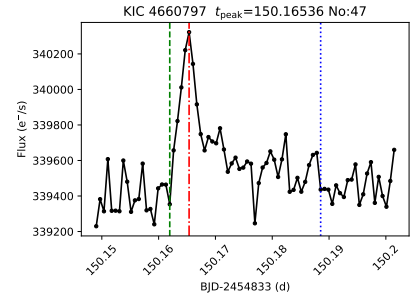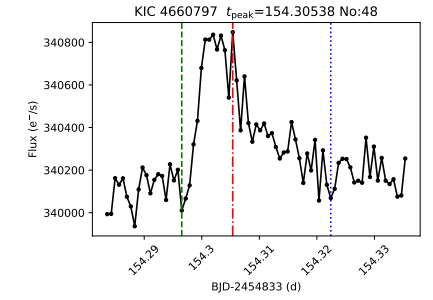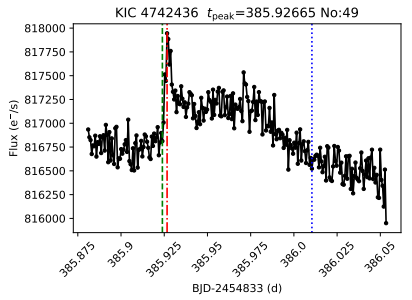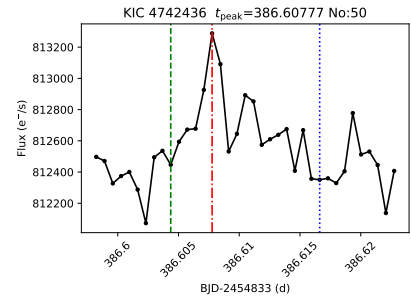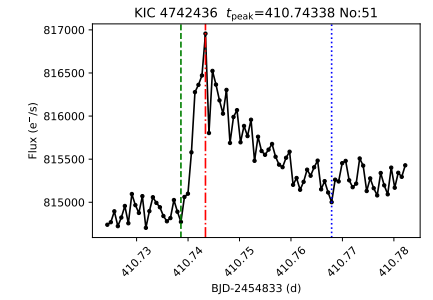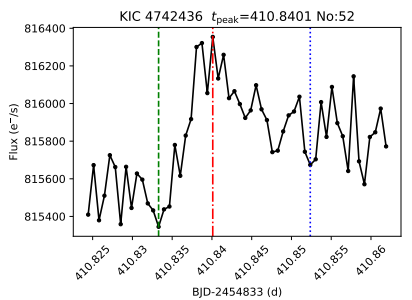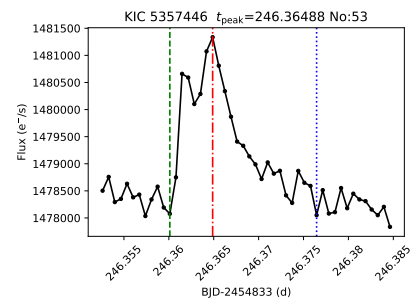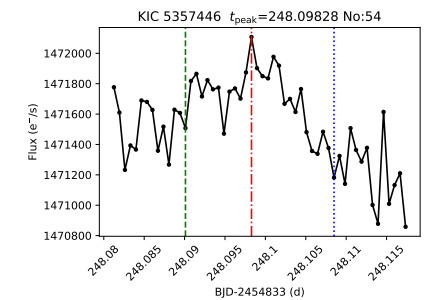

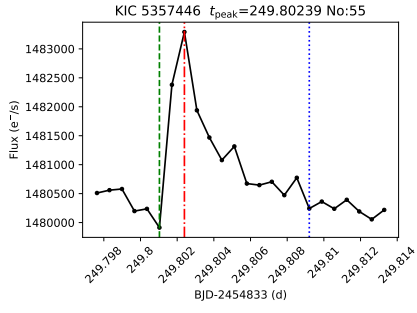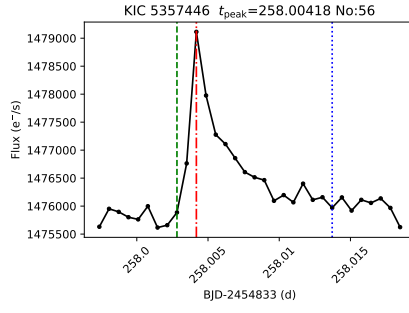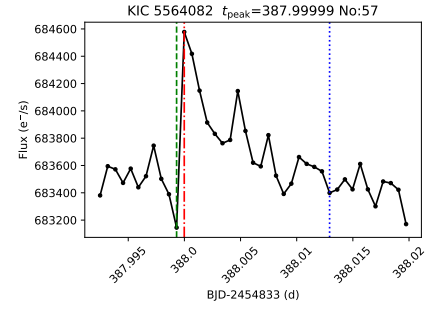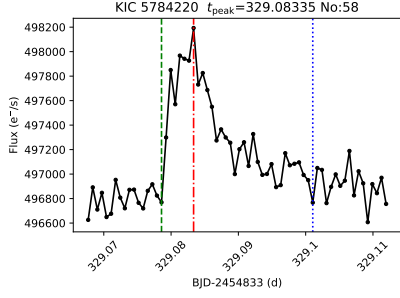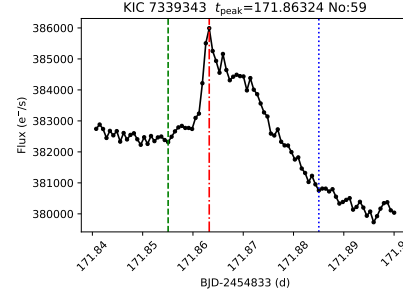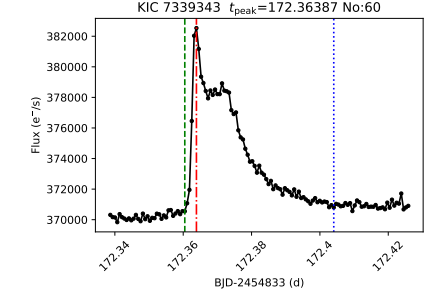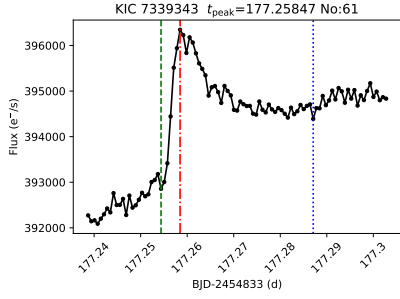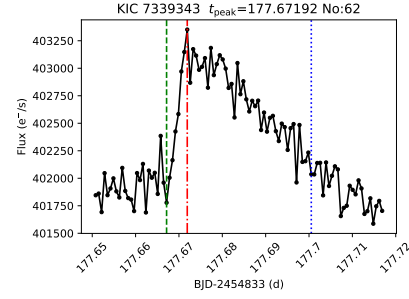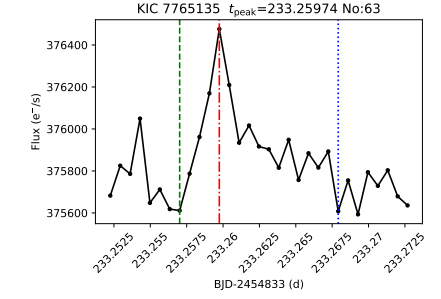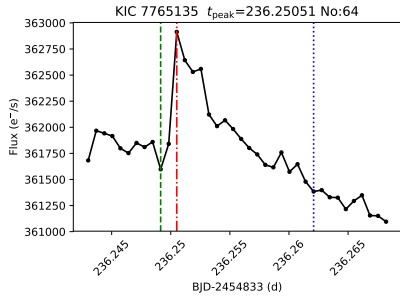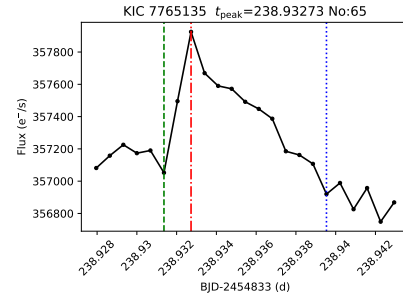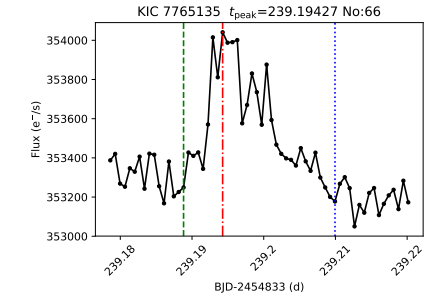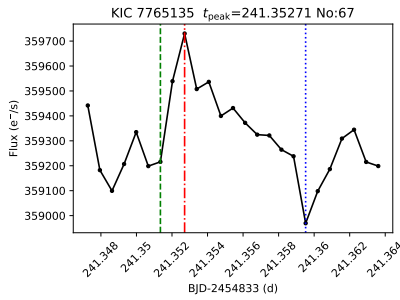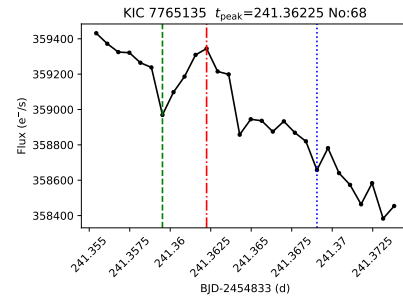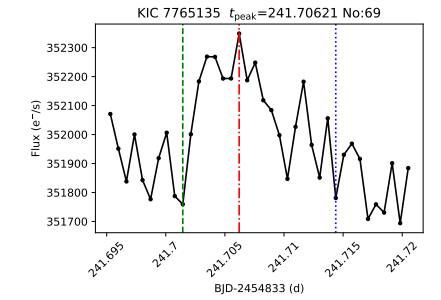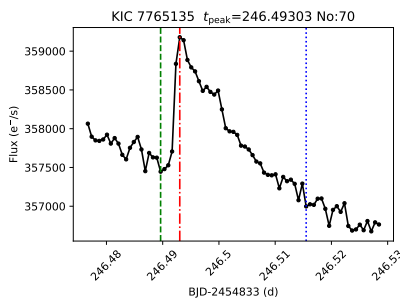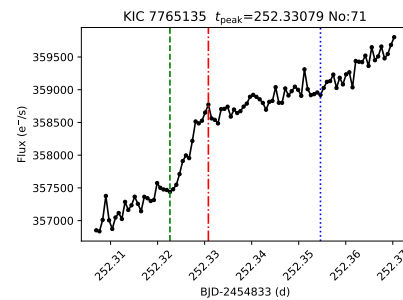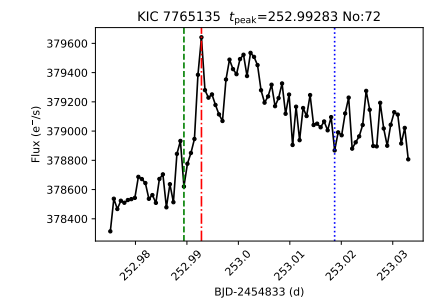

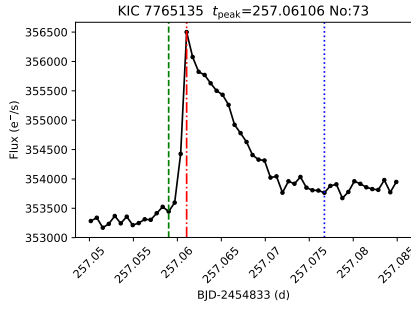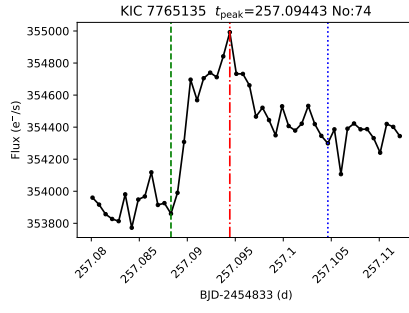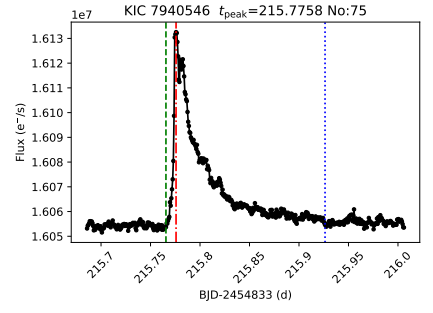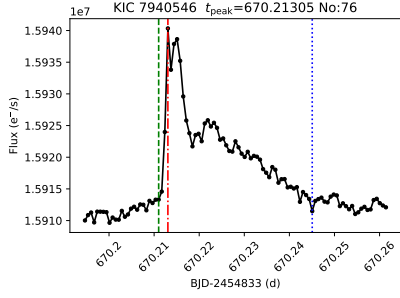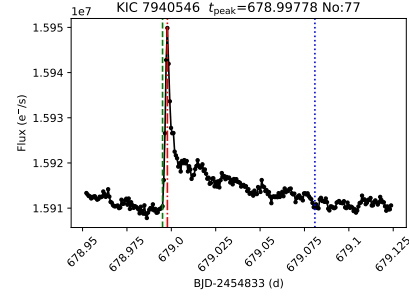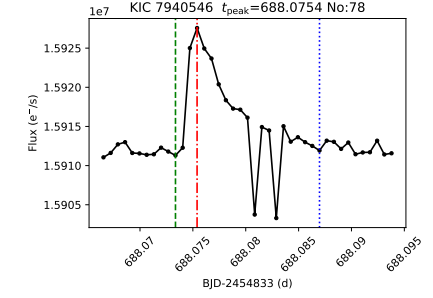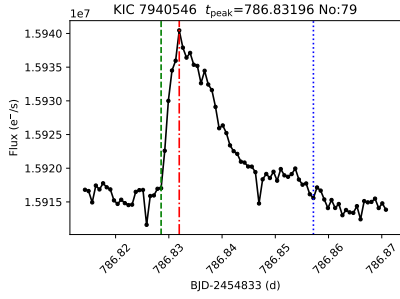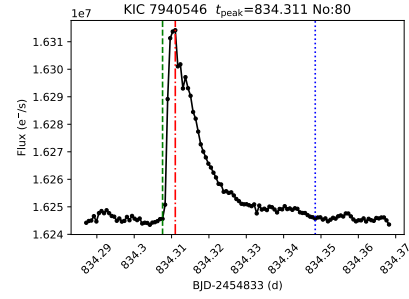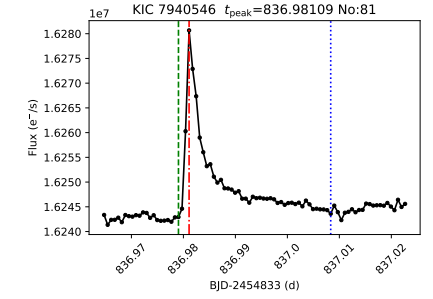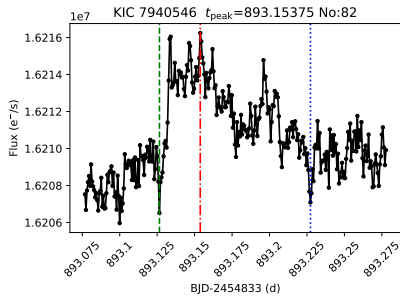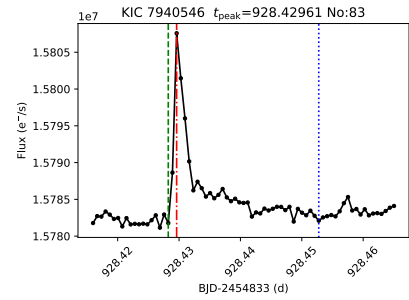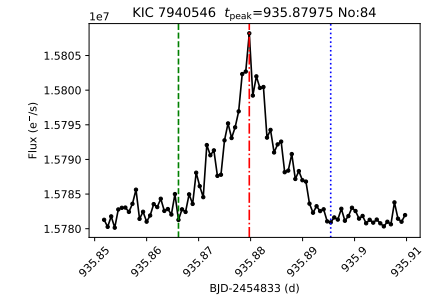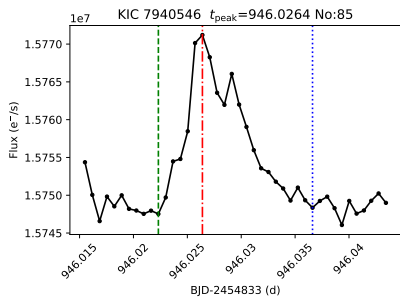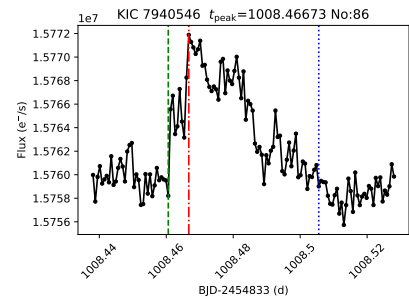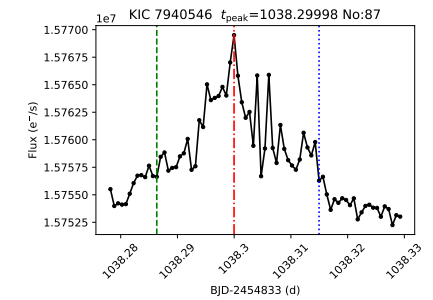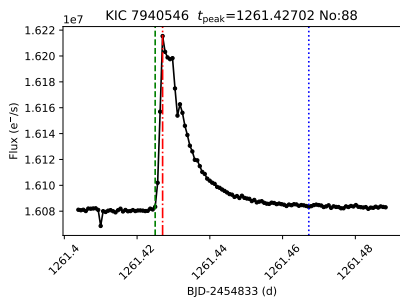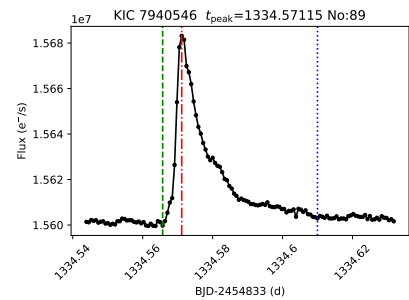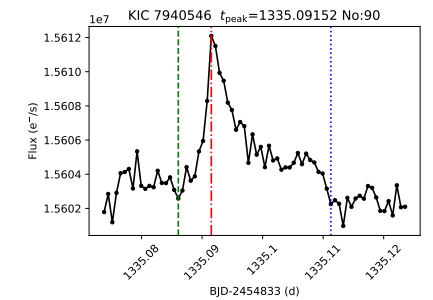

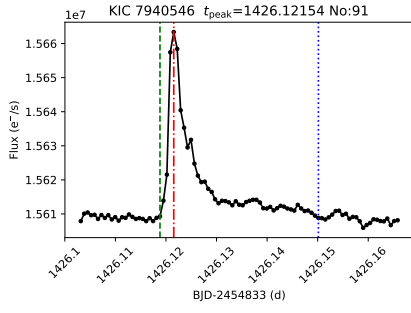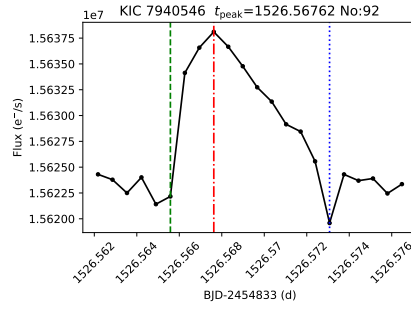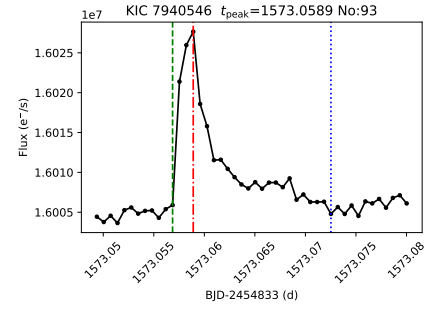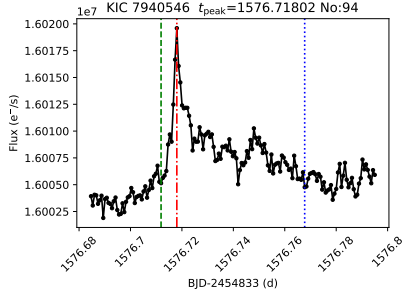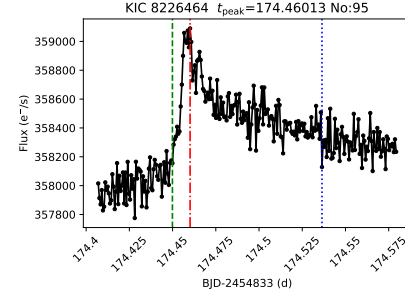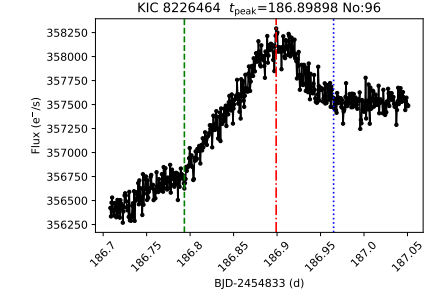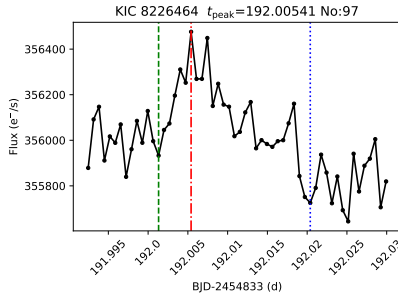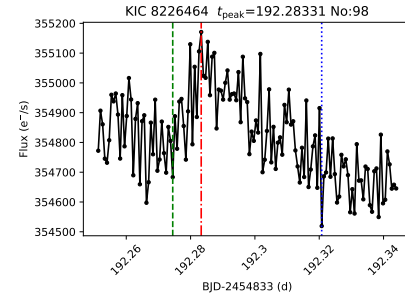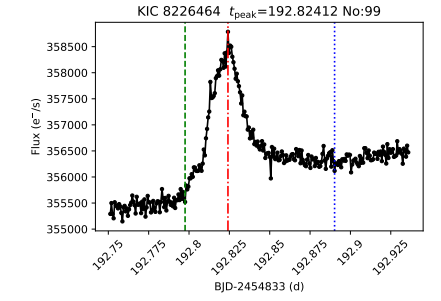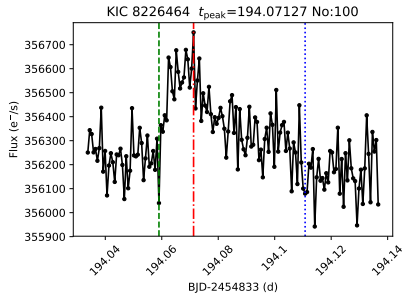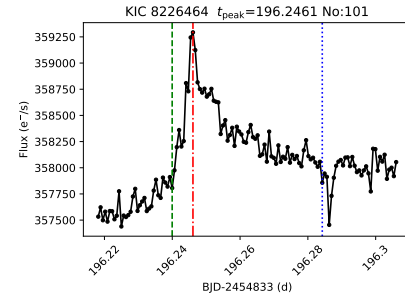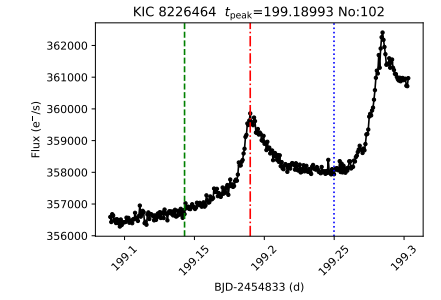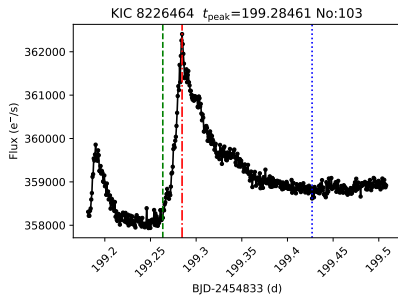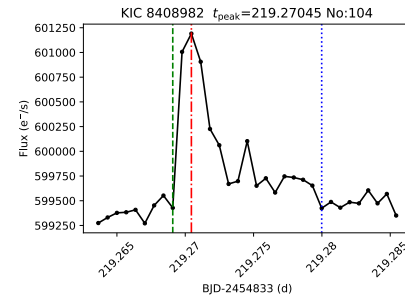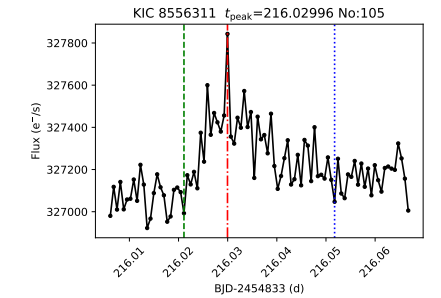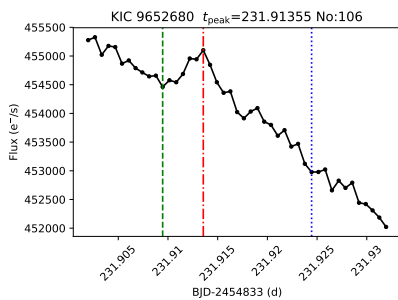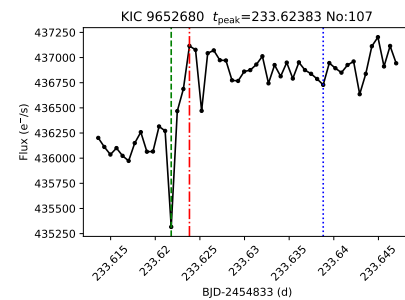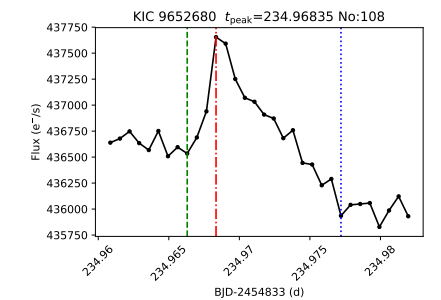



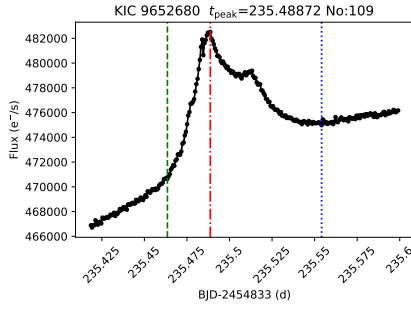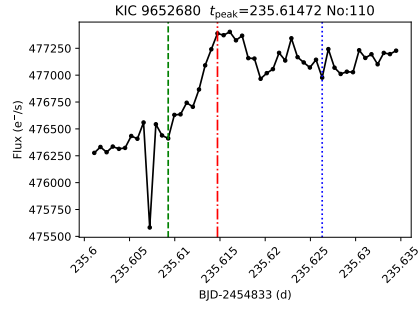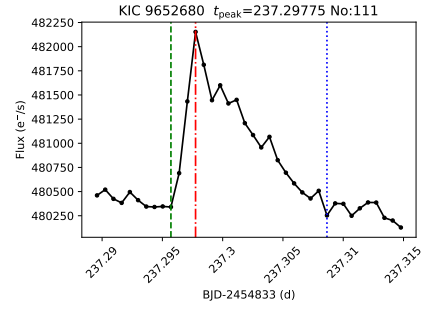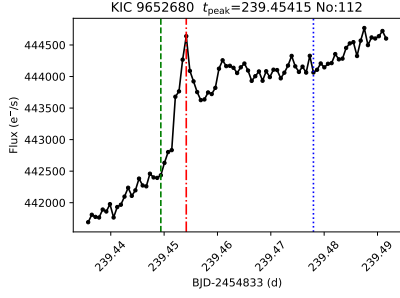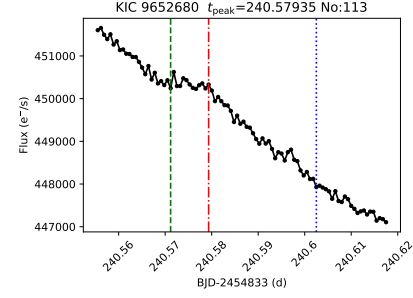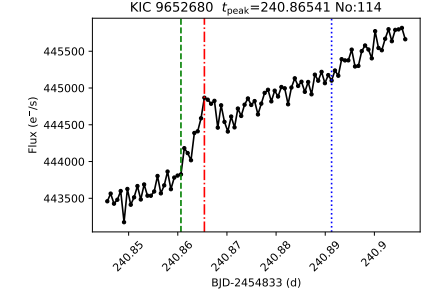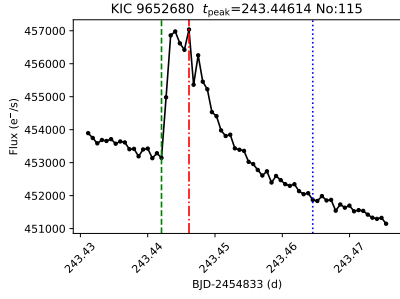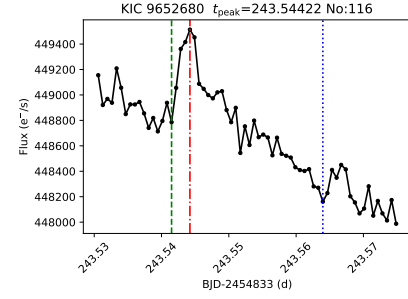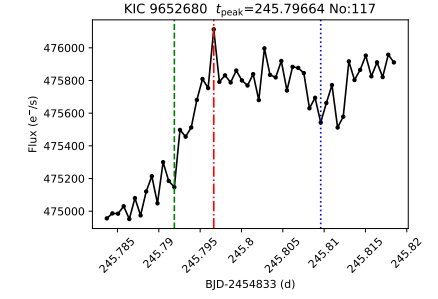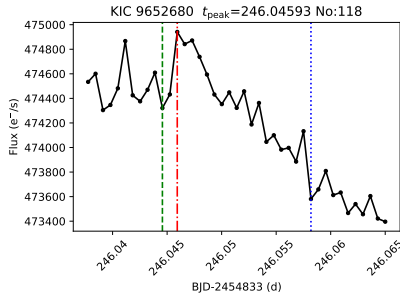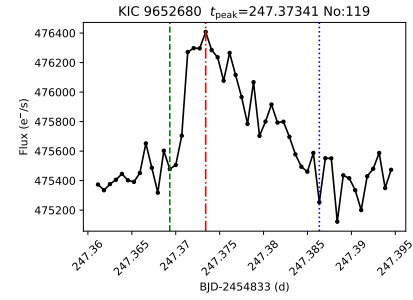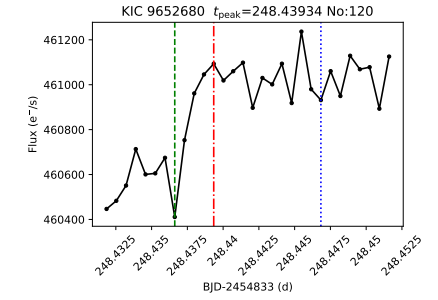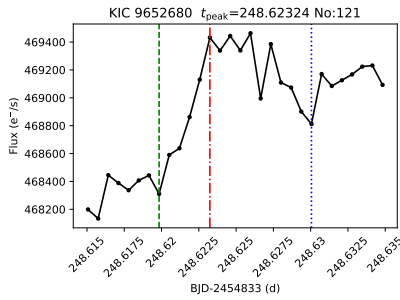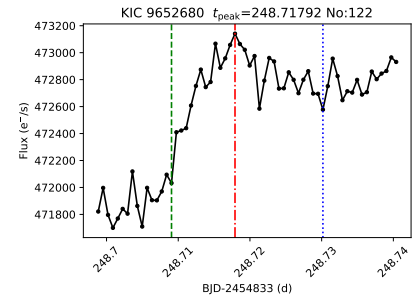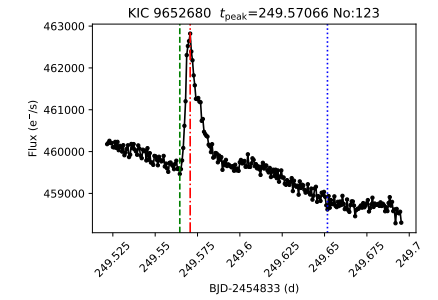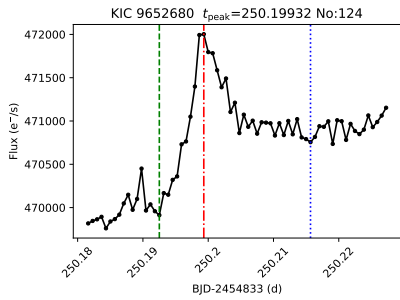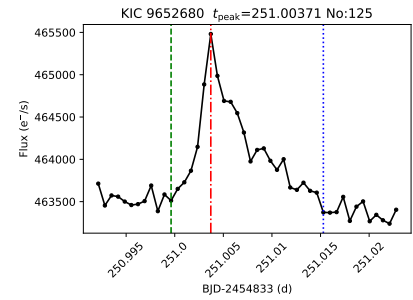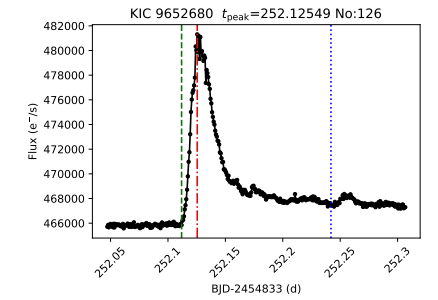



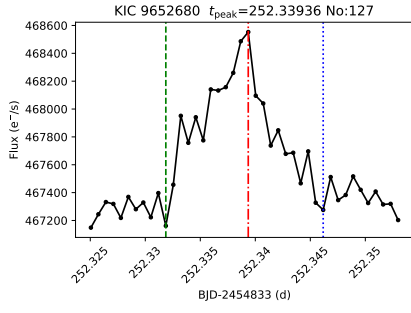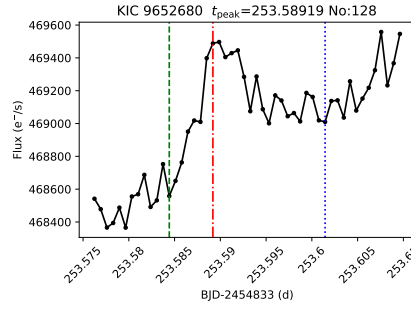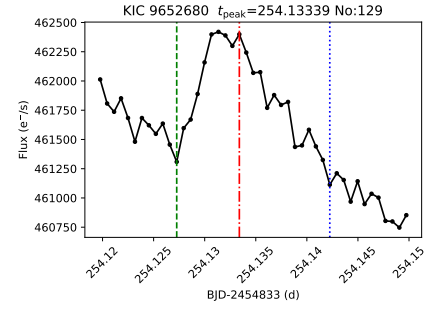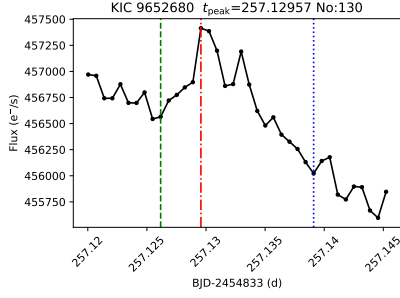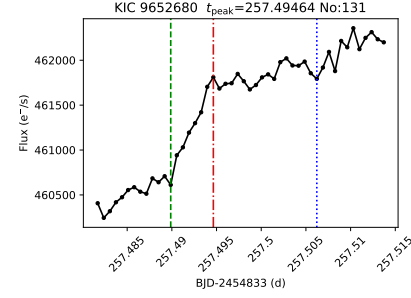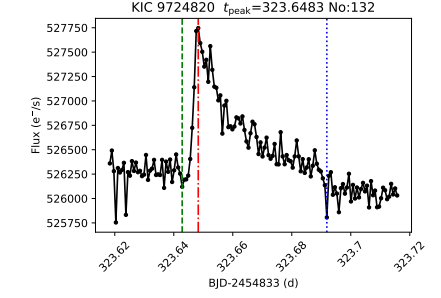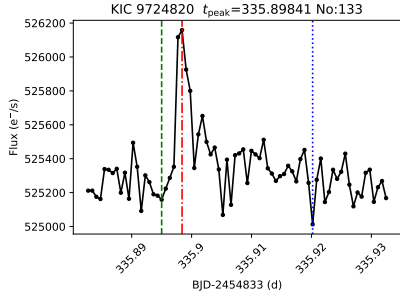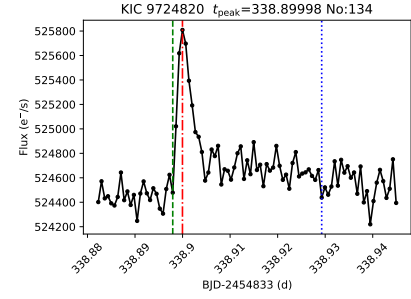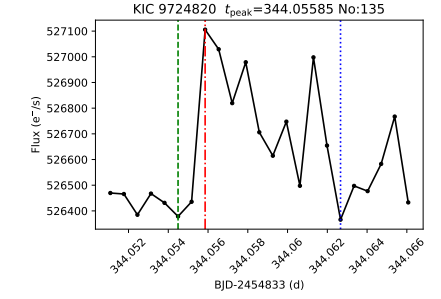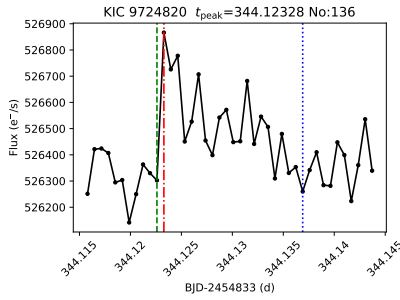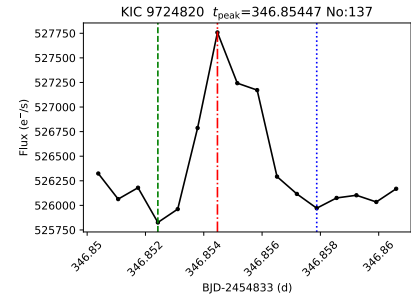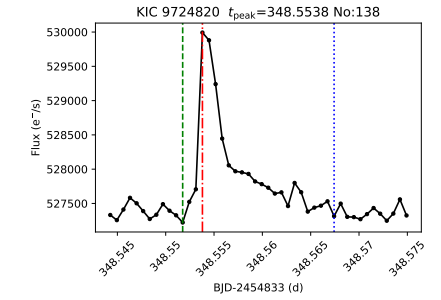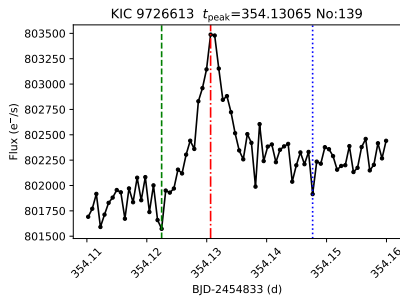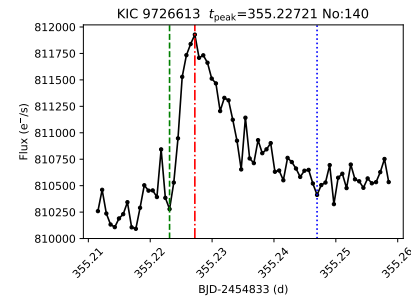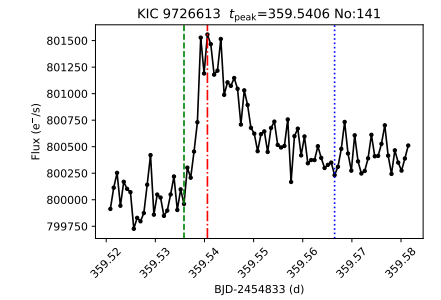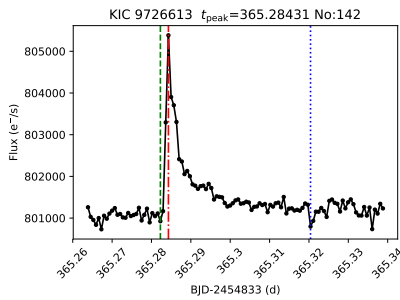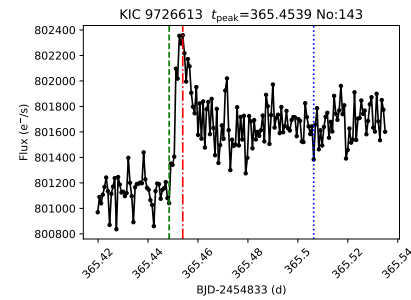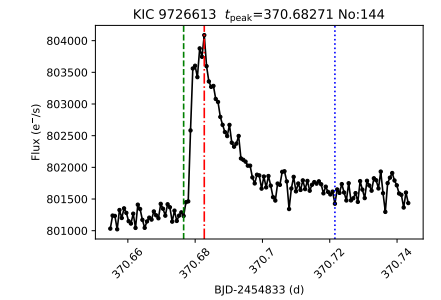

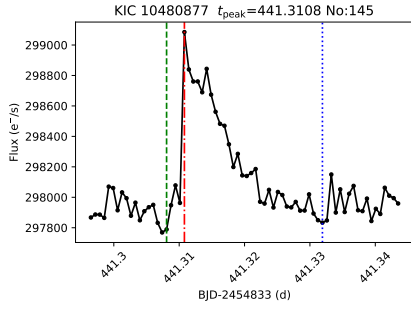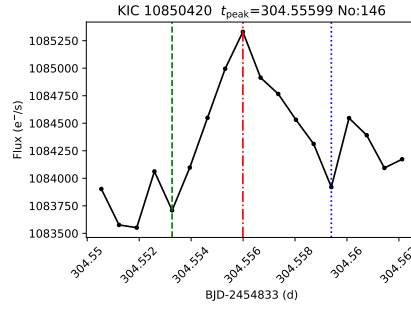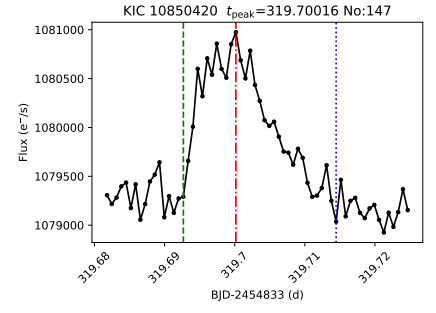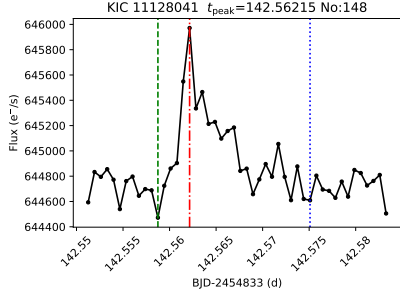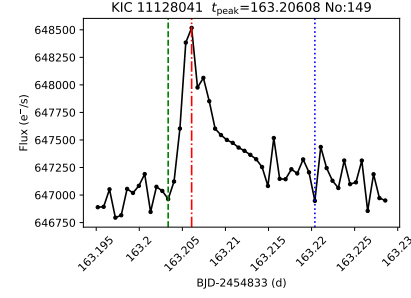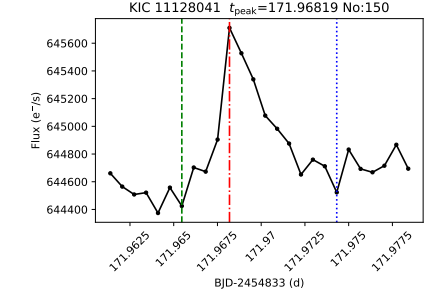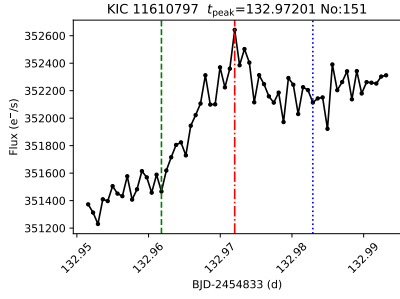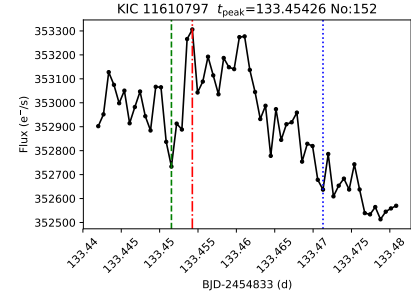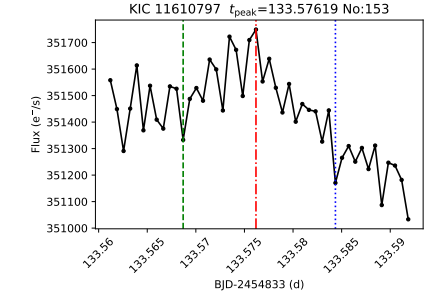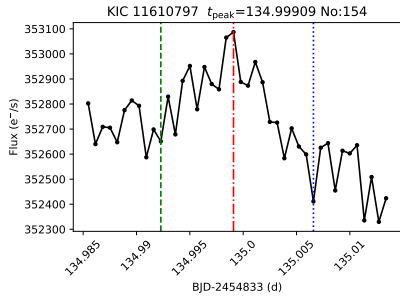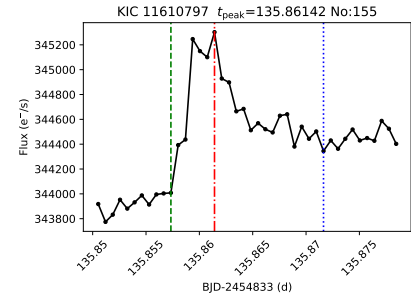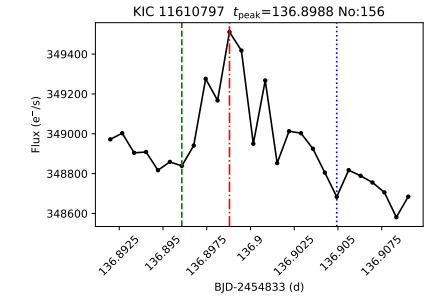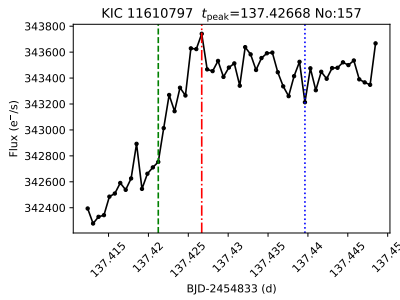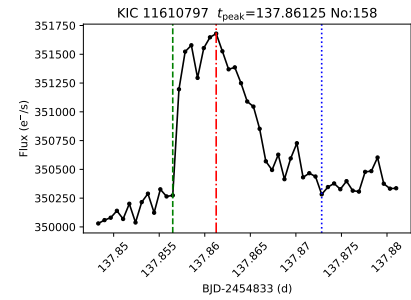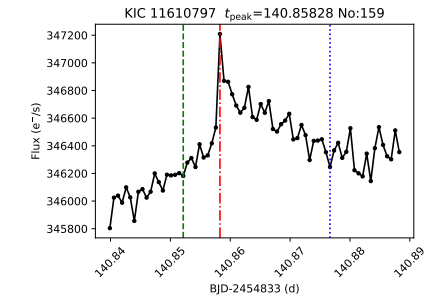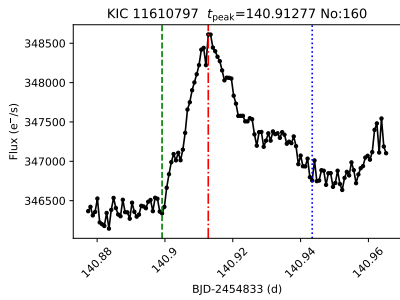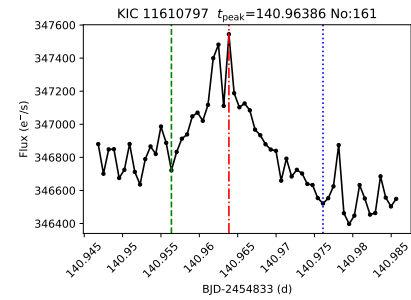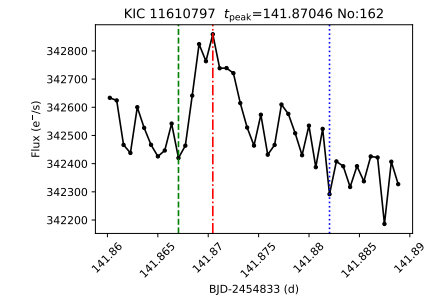

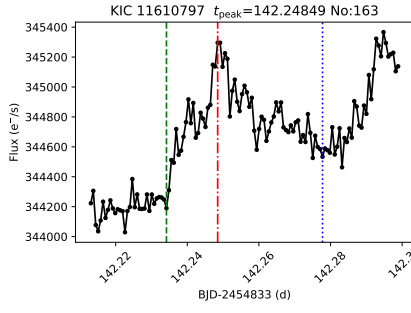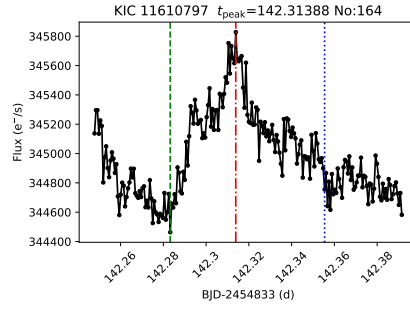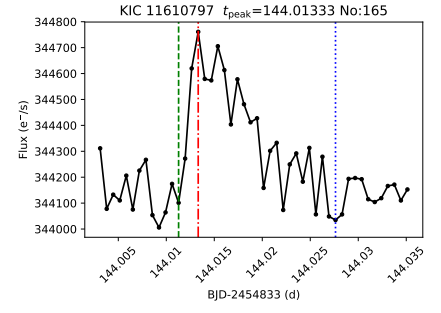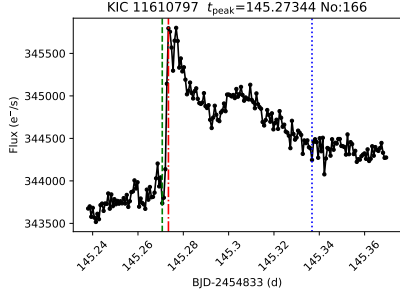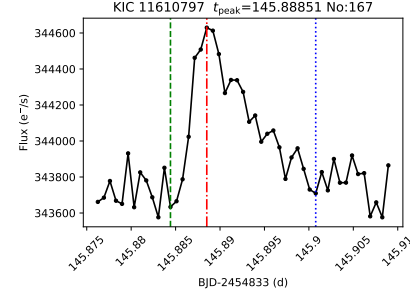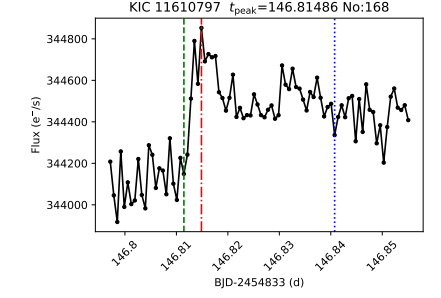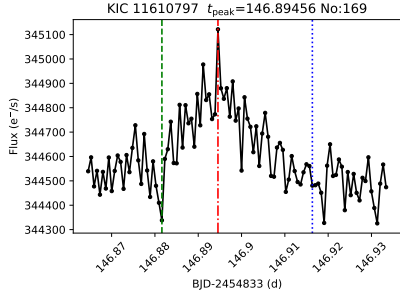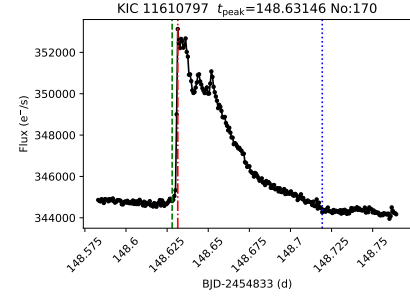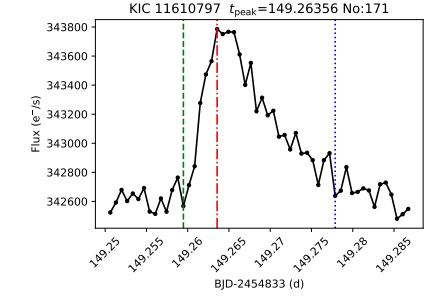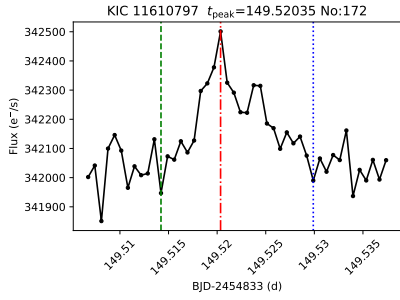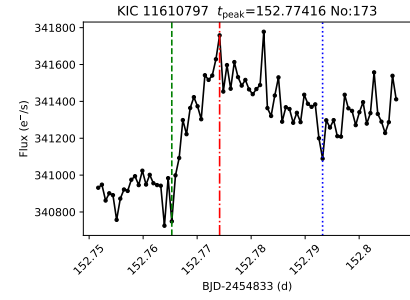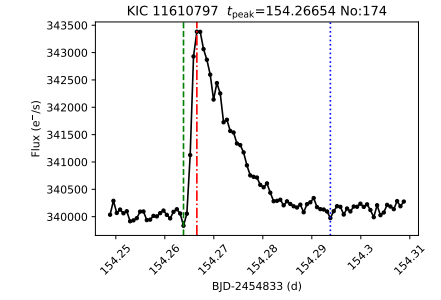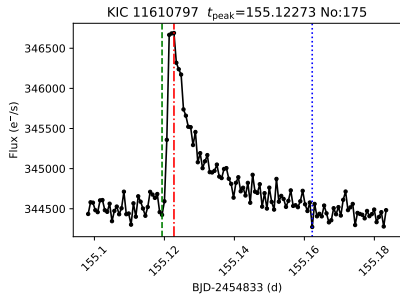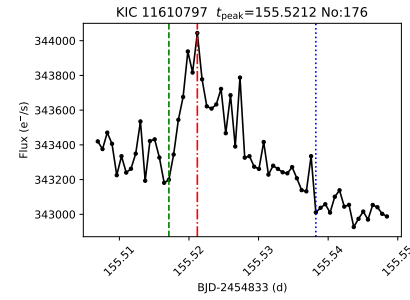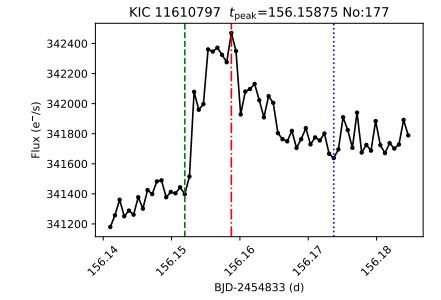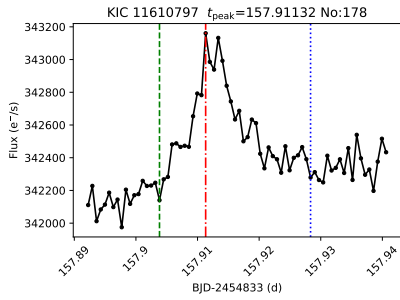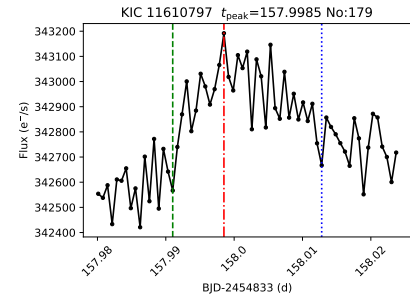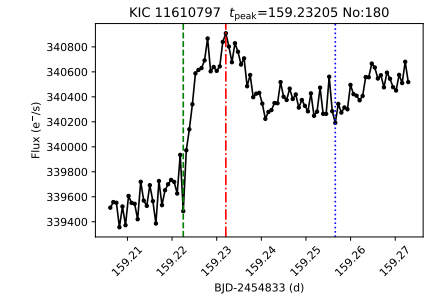

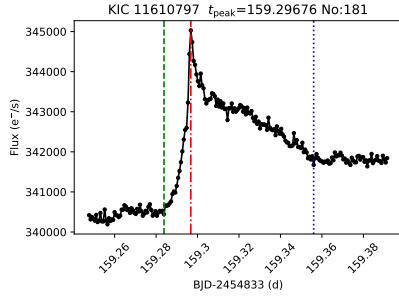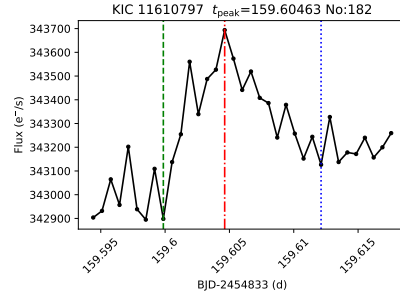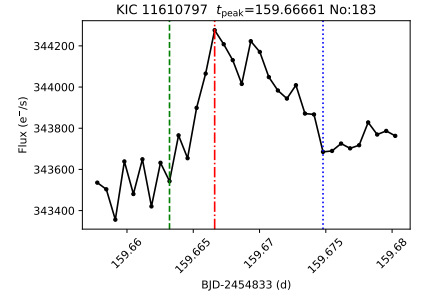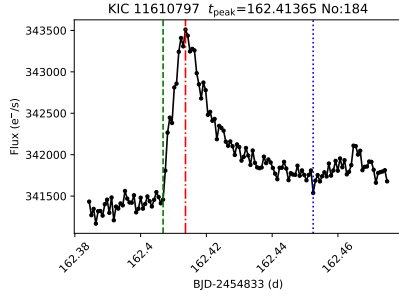

Supplement: Supplementary file 1 [file Plots_of_all_the_flare_samples.pdf]
