# Supplementary material for: Characteristic time of stellar flares on Sun-like stars
Source: arXiv:2105.12375 ancillary file (2021-06-15)
Supplement: Supplementary file 2 [file Table_of_flare_samples.pdf]

Table of Flare Samples

| No. | KIC     | t_start<br>(BJD-2454833) | t_peak<br>(BJD-2454833) | t_end<br>(BJD-2454833) | T_rise<br>(minutes) | T_decay<br>(minutes) |
|-----|---------|--------------------------|-------------------------|------------------------|---------------------|----------------------|
| 1   | 1025986 | 293.77920                | 293.78193               | 293.79691              | 3.9                 | 21.6                 |
| 2   | 1025986 | 294.23621                | 294.23961               | 294.25255              | 4.9                 | 18.6                 |
| 3   | 1025986 | 300.35029                | 300.35506               | 300.36460              | 6.9                 | 13.7                 |
| 4   | 4543412 | 323.75144                | 323.75757               | 323.76575              | 8.8                 | 11.8                 |
| 5   | 4543412 | 323.79163                | 323.79435               | 323.83794              | 3.9                 | 62.8                 |
| 6   | 4543412 | 327.30674                | 327.30878               | 327.33262              | 2.9                 | 34.3                 |
| 7   | 4543412 | 328.32021                | 328.32225               | 328.34404              | 2.9                 | 31.4                 |
| 8   | 4543412 | 328.64985                | 328.65803               | 328.69753              | 11.8                | 56.9                 |
| 9   | 4543412 | 328.72750                | 328.73159               | 328.73908              | 5.9                 | 10.8                 |
| 10  | 4543412 | 329.85879                | 329.86356               | 329.88195              | 6.9                 | 26.5                 |
| 11  | 4543412 | 330.03111                | 330.03656               | 330.04814              | 7.8                 | 16.7                 |
| 12  | 4543412 | 330.80143                | 330.80619               | 330.82186              | 6.9                 | 22.6                 |
| 13  | 4543412 | 330.96966                | 330.97579               | 331.02823              | 8.8                 | 75.5                 |
| 14  | 4543412 | 332.45172                | 332.45580               | 332.46534              | 5.9                 | 13.7                 |
| 15  | 4543412 | 332.61382                | 332.61790               | 332.62948              | 5.9                 | 16.7                 |
| 16  | 4543412 | 332.84471                | 332.84811               | 332.86105              | 4.9                 | 18.6                 |
| 17  | 4543412 | 334.51066                | 334.51816               | 334.52905              | 10.8                | 15.7                 |
| 18  | 4543412 | 334.67753                | 334.67957               | 334.68639              | 2.9                 | 9.8                  |
| 19  | 4543412 | 335.19108                | 335.19516               | 335.21151              | 5.9                 | 23.5                 |
| 20  | 4543412 | 335.65831                | 335.66035               | 335.67329              | 2.9                 | 18.6                 |
| 21  | 4543412 | 335.96957                | 335.97570               | 335.99545              | 8.8                 | 28.4                 |
| 22  | 4543412 | 337.02050                | 337.02254               | 337.04570              | 2.9                 | 33.3                 |
| 23  | 4543412 | 337.07567                | 337.07703               | 337.09065              | 2.0                 | 19.6                 |
| 24  | 4543412 | 337.27931                | 337.28136               | 337.29362              | 2.9                 | 17.7                 |
| 25  | 4543412 | 337.78264                | 337.78673               | 337.80308              | 5.9                 | 23.5                 |
| 26  | 4543412 | 338.74707                | 338.75525               | 338.76887              | 11.8                | 19.6                 |
| 27  | 4543412 | 341.34001                | 341.34273               | 341.35363              | 3.9                 | 15.7                 |
| 28  | 4543412 | 341.36930                | 341.37406               | 341.38292              | 6.9                 | 12.8                 |
| 29  | 4543412 | 341.45307                | 341.45648               | 341.46193              | 4.9                 | 7.8                  |
| 30  | 4543412 | 342.10420                | 342.11305               | 342.14098              | 12.8                | 40.2                 |
| 31  | 4543412 | 342.19955                | 342.20160               | 342.21590              | 2.9                 | 20.6                 |
| 32  | 4543412 | 343.37240                | 343.37717               | 343.38739              | 6.9                 | 14.7                 |
| 33  | 4543412 | 344.32185                | 344.32458               | 344.35046              | 3.9                 | 37.3                 |
| 34  | 4543412 | 344.37362                | 344.37975               | 344.39609              | 8.8                 | 23.5                 |
| 35  | 4543412 | 345.98510                | 345.98714               | 345.99940              | 2.9                 | 17.7                 |
| 36  | 4543412 | 346.13290                | 346.13903               | 346.16218              | 8.8                 | 33.3                 |
| 37  | 4543412 | 347.89286                | 347.89558               | 347.89899              | 3.9                 | 4.9                  |
| 38  | 4543412 | 347.90035                | 347.90444               | 347.90852              | 5.9                 | 5.9                  |
| 39  | 4543412 | 348.14350                | 348.14759               | 348.15508              | 5.9                 | 10.8                 |
| 40  | 4543412 | 348.51947                | 348.52219               | 348.54603              | 3.9                 | 34.3                 |
| 41  | 4543412 | 348.73538                | 348.74423               | 348.76194              | 12.8                | 25.5                 |
| 42  | 4543412 | 349.11203                | 349.11339               | 349.13042              | 2.0                 | 24.5                 |
| 43  | 4660797 | 134.84357                | 134.84425               | 134.85243              | 1.0                 | 11.8                 |
| 44  | 4660797 | 135.25022                | 135.25090               | 135.25771              | 1.0                 | 9.8                  |
| 45  | 4660797 | 144.63035                | 144.63239               | 144.64874              | 2.9                 | 23.5                 |
| 46  | 4660797 | 147.68462                | 147.69143               | 147.71187              | 9.8                 | 29.4                 |
| 47  | 4660797 | 150.16196                | 150.16536               | 150.18852              | 4.9                 | 33.3                 |
| 48  | 4660797 | 154.29653                | 154.30538               | 154.32241              | 12.8                | 24.5                 |
| 49  | 4742436 | 385.92393                | 385.92665               | 386.01043              | 3.9                 | 120.6                |
| 50  | 4742436 | 386.60436                | 386.60777               | 386.61662              | 4.9                 | 12.8                 |
| 51  | 4742436 | 410.73862                | 410.74338               | 410.76790              | 6.9                 | 35.3                 |
| 52  | 4742436 | 410.83329                | 410.84010               | 410.85236              | 9.8                 | 17.7                 |
| 53  | 5357446 | 246.36011                | 246.36488               | 246.37646              | 6.9                 | 16.7                 |
| 54  | 5357446 | 248.09011                | 248.09828               | 248.10850              | 11.8                | 14.7                 |
| 55  | 5357446 | 249.80103                | 249.80239               | 249.80921              | 2.0                 | 9.8                  |
| 56  | 5357446 | 258.00282                | 258.00418               | 258.01372              | 2.0                 | 13.7                 |
| 57  | 5564082 | 387.99931                | 387.99999               | 388.01293              | 1.0                 | 18.6                 |
| 58  | 5784220 | 329.07858                | 329.08335               | 329.10105              | 6.9                 | 25.5                 |
| 59  | 7339343 | 171.85506                | 171.86324               | 171.88503              | 11.8                | 31.4                 |

|     |         |            |            |            |       |       |
|-----|---------|------------|------------|------------|-------|-------|
| 60  | 7339343 | 172.36046  | 172.36387  | 172.40406  | 4.9   | 57.9  |
| 61  | 7339343 | 177.25438  | 177.25847  | 177.28708  | 5.9   | 41.2  |
| 62  | 7339343 | 177.66715  | 177.67192  | 177.70052  | 6.9   | 41.2  |
| 63  | 7765135 | 233.25702  | 233.25974  | 233.26792  | 3.9   | 11.8  |
| 64  | 7765135 | 236.24915  | 236.25051  | 236.26209  | 2.0   | 16.7  |
| 65  | 7765135 | 238.93136  | 238.93273  | 238.93954  | 2.0   | 9.8   |
| 66  | 7765135 | 239.18882  | 239.19427  | 239.20994  | 7.8   | 22.6  |
| 67  | 7765135 | 241.35135  | 241.35271  | 241.35952  | 2.0   | 9.8   |
| 68  | 7765135 | 241.35952  | 241.36225  | 241.36906  | 3.9   | 9.8   |
| 69  | 7765135 | 241.70144  | 241.70621  | 241.71438  | 6.9   | 11.8  |
| 70  | 7765135 | 246.48963  | 246.49303  | 246.51551  | 4.9   | 32.4  |
| 71  | 7765135 | 252.32262  | 252.33079  | 252.35463  | 11.8  | 34.3  |
| 72  | 7765135 | 252.98942  | 252.99283  | 253.01871  | 4.9   | 37.3  |
| 73  | 7765135 | 257.05901  | 257.06106  | 257.07672  | 2.9   | 22.6  |
| 74  | 7765135 | 257.08830  | 257.09443  | 257.10465  | 8.8   | 14.7  |
| 75  | 7940546 | 215.76558  | 215.77580  | 215.92632  | 14.7  | 216.8 |
| 76  | 7940546 | 670.21101  | 670.21305  | 670.24507  | 2.9   | 46.1  |
| 77  | 7940546 | 678.99506  | 678.99778  | 679.08088  | 3.9   | 119.7 |
| 78  | 7940546 | 688.07336  | 688.07540  | 688.08698  | 2.9   | 16.7  |
| 79  | 7940546 | 786.82855  | 786.83196  | 786.85716  | 4.9   | 36.3  |
| 80  | 7940546 | 834.30759  | 834.31100  | 834.34846  | 4.9   | 53.9  |
| 81  | 7940546 | 836.97905  | 836.98109  | 837.00834  | 2.9   | 39.2  |
| 82  | 7940546 | 893.12651  | 893.15375  | 893.22732  | 39.2  | 105.9 |
| 83  | 7940546 | 928.42824  | 928.42961  | 928.45276  | 2.0   | 33.3  |
| 84  | 7940546 | 935.86612  | 935.87975  | 935.89541  | 19.6  | 22.6  |
| 85  | 7940546 | 946.02231  | 946.02640  | 946.03662  | 5.9   | 14.7  |
| 86  | 7940546 | 1008.46060 | 1008.46673 | 1008.50555 | 8.8   | 55.9  |
| 87  | 7940546 | 1038.28636 | 1038.29998 | 1038.31496 | 19.6  | 21.6  |
| 88  | 7940546 | 1261.42497 | 1261.42702 | 1261.46720 | 2.9   | 57.9  |
| 89  | 7940546 | 1334.56570 | 1334.57115 | 1334.60998 | 7.8   | 55.9  |
| 90  | 7940546 | 1335.08607 | 1335.09152 | 1335.11127 | 7.8   | 28.4  |
| 91  | 7940546 | 1426.11882 | 1426.12154 | 1426.15015 | 3.9   | 41.2  |
| 92  | 7940546 | 1526.56558 | 1526.56762 | 1526.57307 | 2.9   | 7.8   |
| 93  | 7940546 | 1573.05686 | 1573.05890 | 1573.07253 | 2.9   | 19.6  |
| 94  | 7940546 | 1576.71189 | 1576.71802 | 1576.76775 | 8.8   | 71.6  |
| 95  | 8226464 | 174.44991  | 174.46013  | 174.53642  | 14.7  | 109.9 |
| 96  | 8226464 | 186.79340  | 186.89898  | 186.96505  | 152.0 | 95.1  |
| 97  | 8226464 | 192.00132  | 192.00541  | 192.02039  | 5.9   | 21.6  |
| 98  | 8226464 | 192.27445  | 192.28331  | 192.32077  | 12.8  | 53.9  |
| 99  | 8226464 | 192.79756  | 192.82412  | 192.89019  | 38.3  | 95.1  |
| 100 | 8226464 | 194.05901  | 194.07127  | 194.11077  | 17.7  | 56.9  |
| 101 | 8226464 | 196.23997  | 196.24610  | 196.28425  | 8.8   | 54.9  |
| 102 | 8226464 | 199.14293  | 199.18993  | 199.24987  | 67.7  | 86.3  |
| 103 | 8226464 | 199.26349  | 199.28461  | 199.42696  | 30.4  | 205.0 |
| 104 | 8408982 | 219.26909  | 219.27045  | 219.27998  | 2.0   | 13.7  |
| 105 | 8556311 | 216.02110  | 216.02996  | 216.05176  | 12.8  | 31.4  |
| 106 | 9652680 | 231.90947  | 231.91355  | 231.92445  | 5.9   | 15.7  |
| 107 | 9652680 | 233.62179  | 233.62383  | 233.63881  | 2.9   | 21.6  |
| 108 | 9652680 | 234.96630  | 234.96835  | 234.97720  | 2.9   | 12.8  |
| 109 | 9652680 | 235.46352  | 235.48872  | 235.55410  | 36.3  | 94.2  |
| 110 | 9652680 | 235.60927  | 235.61472  | 235.62630  | 7.8   | 16.7  |
| 111 | 9652680 | 237.29571  | 237.29775  | 237.30865  | 2.9   | 15.7  |
| 112 | 9652680 | 239.44938  | 239.45415  | 239.47799  | 6.9   | 34.3  |
| 113 | 9652680 | 240.57117  | 240.57935  | 240.60250  | 11.8  | 33.3  |
| 114 | 9652680 | 240.86065  | 240.86541  | 240.89130  | 6.9   | 37.3  |
| 115 | 9652680 | 243.44205  | 243.44614  | 243.46453  | 5.9   | 26.5  |
| 116 | 9652680 | 243.54149  | 243.54422  | 243.56397  | 3.9   | 28.4  |
| 117 | 9652680 | 245.79188  | 245.79664  | 245.80959  | 6.9   | 18.6  |
| 118 | 9652680 | 246.04457  | 246.04593  | 246.05819  | 2.0   | 17.7  |
| 119 | 9652680 | 247.36932  | 247.37341  | 247.38635  | 5.9   | 18.6  |
| 120 | 9652680 | 248.43662  | 248.43934  | 248.44684  | 3.9   | 10.8  |
| 121 | 9652680 | 248.61984  | 248.62324  | 248.63005  | 4.9   | 9.8   |
| 122 | 9652680 | 248.70906  | 248.71792  | 248.73018  | 12.8  | 17.7  |
| 123 | 9652680 | 249.56453  | 249.57066  | 249.65171  | 8.8   | 116.7 |
| 124 | 9652680 | 250.19251  | 250.19932  | 250.21567  | 9.8   | 23.5  |
| 125 | 9652680 | 250.99962  | 251.00371  | 251.01529  | 5.9   | 16.7  |

|     |          |           |           |           |      |       |
|-----|----------|-----------|-----------|-----------|------|-------|
| 126 | 9652680  | 252.11187 | 252.12549 | 252.24196 | 19.6 | 167.7 |
| 127 | 9652680  | 252.33187 | 252.33936 | 252.34617 | 10.8 | 9.8   |
| 128 | 9652680  | 253.58442 | 253.58919 | 253.60145 | 6.9  | 17.7  |
| 129 | 9652680  | 254.12726 | 254.13339 | 254.14225 | 8.8  | 12.8  |
| 130 | 9652680  | 257.12616 | 257.12957 | 257.13910 | 4.9  | 13.7  |
| 131 | 9652680  | 257.48987 | 257.49464 | 257.50622 | 6.9  | 16.7  |
| 132 | 9724820  | 323.64285 | 323.64830 | 323.69189 | 7.8  | 62.8  |
| 133 | 9724820  | 335.89500 | 335.89841 | 335.92020 | 4.9  | 31.4  |
| 134 | 9724820  | 338.89794 | 338.89998 | 338.92927 | 2.9  | 42.2  |
| 135 | 9724820  | 344.05449 | 344.05585 | 344.06266 | 2.0  | 9.8   |
| 136 | 9724820  | 344.12260 | 344.12328 | 344.13690 | 1.0  | 19.6  |
| 137 | 9724820  | 346.85243 | 346.85447 | 346.85787 | 2.9  | 4.9   |
| 138 | 9724820  | 348.55176 | 348.55380 | 348.56742 | 2.9  | 19.6  |
| 139 | 9726613  | 354.12248 | 354.13065 | 354.14768 | 11.8 | 24.5  |
| 140 | 9726613  | 355.22313 | 355.22721 | 355.24696 | 5.9  | 28.4  |
| 141 | 9726613  | 359.53583 | 359.54060 | 359.56648 | 6.9  | 37.3  |
| 142 | 9726613  | 365.28226 | 365.28431 | 365.32040 | 2.9  | 52.0  |
| 143 | 9726613  | 365.44845 | 365.45390 | 365.50634 | 7.8  | 75.5  |
| 144 | 9726613  | 370.67658 | 370.68271 | 370.72153 | 8.8  | 55.9  |
| 145 | 10480877 | 441.30807 | 441.31080 | 441.33191 | 3.9  | 30.4  |
| 146 | 10850420 | 304.55327 | 304.55599 | 304.55940 | 3.9  | 4.9   |
| 147 | 10850420 | 319.69267 | 319.70016 | 319.71447 | 10.8 | 20.6  |
| 148 | 11128041 | 142.55875 | 142.56215 | 142.57509 | 4.9  | 18.6  |
| 149 | 11128041 | 163.20335 | 163.20608 | 163.22038 | 3.9  | 20.6  |
| 150 | 11128041 | 171.96546 | 171.96819 | 171.97432 | 3.9  | 8.8   |
| 151 | 11610797 | 132.96180 | 132.97201 | 132.98291 | 14.7 | 15.7  |
| 152 | 11610797 | 133.45154 | 133.45426 | 133.47129 | 3.9  | 24.5  |
| 153 | 11610797 | 133.56869 | 133.57619 | 133.58436 | 10.8 | 11.8  |
| 154 | 11610797 | 134.99228 | 134.99909 | 135.00659 | 9.8  | 10.8  |
| 155 | 11610797 | 135.85733 | 135.86142 | 135.87164 | 5.9  | 14.7  |
| 156 | 11610797 | 136.89607 | 136.89880 | 136.90493 | 3.9  | 8.8   |
| 157 | 11610797 | 137.42124 | 137.42668 | 137.43963 | 7.8  | 18.6  |
| 158 | 11610797 | 137.85649 | 137.86125 | 137.87283 | 6.9  | 16.7  |
| 159 | 11610797 | 140.85215 | 140.85828 | 140.87667 | 8.8  | 26.5  |
| 160 | 11610797 | 140.89915 | 140.91277 | 140.94342 | 19.6 | 44.1  |
| 161 | 11610797 | 140.95636 | 140.96386 | 140.97612 | 10.8 | 17.7  |
| 162 | 11610797 | 141.86705 | 141.87046 | 141.88203 | 4.9  | 16.7  |
| 163 | 11610797 | 142.23418 | 142.24849 | 142.27778 | 20.6 | 42.2  |
| 164 | 11610797 | 142.28323 | 142.31388 | 142.35543 | 44.1 | 59.8  |
| 165 | 11610797 | 144.01128 | 144.01333 | 144.02763 | 2.9  | 20.6  |
| 166 | 11610797 | 145.27071 | 145.27344 | 145.33678 | 3.9  | 91.2  |
| 167 | 11610797 | 145.88442 | 145.88851 | 145.90077 | 5.9  | 17.7  |
| 168 | 11610797 | 146.81146 | 146.81486 | 146.84074 | 4.9  | 37.3  |
| 169 | 11610797 | 146.88161 | 146.89456 | 146.91635 | 18.6 | 31.4  |
| 170 | 11610797 | 148.62806 | 148.63146 | 148.71933 | 4.9  | 126.5 |
| 171 | 11610797 | 149.25948 | 149.26356 | 149.27787 | 5.9  | 20.6  |
| 172 | 11610797 | 149.51422 | 149.52035 | 149.52989 | 8.8  | 13.7  |
| 173 | 11610797 | 152.76531 | 152.77416 | 152.79323 | 12.8 | 27.5  |
| 174 | 11610797 | 154.26382 | 154.26654 | 154.29379 | 3.9  | 39.2  |
| 175 | 11610797 | 155.11933 | 155.12273 | 155.16224 | 4.9  | 56.9  |
| 176 | 11610797 | 155.51711 | 155.52120 | 155.53823 | 5.9  | 24.5  |
| 177 | 11610797 | 156.15194 | 156.15875 | 156.17373 | 9.8  | 21.6  |
| 178 | 11610797 | 157.90383 | 157.91132 | 157.92835 | 10.8 | 24.5  |
| 179 | 11610797 | 157.99101 | 157.99850 | 158.01281 | 10.8 | 20.6  |
| 180 | 11610797 | 159.22251 | 159.23205 | 159.25657 | 13.7 | 35.3  |
| 181 | 11610797 | 159.28381 | 159.29676 | 159.35602 | 18.6 | 85.3  |
| 182 | 11610797 | 159.59986 | 159.60463 | 159.61212 | 6.9  | 10.8  |
| 183 | 11610797 | 159.66321 | 159.66661 | 159.67479 | 4.9  | 11.8  |
| 184 | 11610797 | 162.40684 | 162.41365 | 162.45247 | 9.8  | 55.9  |
